# Supplementary material for: ZeRO-Infinity: Breaking the GPU Memory Wall for Extreme Scale Deep Learning
Source: arXiv:2104.07857 source file (2021-04-16)
Supplement: Supplementary file 1 [file appendix2.tex]

Our implementation of ZeRO was written in Python on top of
PyTorch 1.2. We used torch.distributed and NVIDIA NCCL 2.4.8 for inter-GPU
communication. We used NVIDIA Megatron-LM as our baseline, and 
integrated it with our DeepSpeed Library and ZeRO implementation for all of our 
experiments. All of our code is open source and available with detailed tutorials on 
how to use it, see ARTIFACT AVAILABILITY for details.

To offer full reproducibility of our results, we provide the model configurations
(number of layers, hidden size, and attention heads), batch sizes, and number of GPUs 
we used for every experiment in Tables 1-6 below.

%START_LATEX
\begin{table*}[!ht]
\begin{tabular}{|l|l|l|l|l|l|l|l|l|}
\hline
\multicolumn{9}{|c|}{Figure 2} \\ \hline
Model size & ZeRO/Baseline & Number of GPUs & MP & Layers & Hidden size & Attention head & Batch size & Total batch size \\ \hline
1.5B & ZeRO & 400 & 1 & 48 & 1600 & 16 & 24 & 9600 \\ \hline
1.5B & Baseline & 400 & 2 & 48 & 1600 & 16 & 16 & 3200 \\ \hline
8B & ZeRO & 400 & 4 & 72 & 3072 & 24 & 64 & 6400 \\ \hline
8B & Baseline & 400 & 8 & 72 & 3072 & 24 & 8 & 400 \\ \hline
20B & ZeRO & 400 & 4 & 98 & 4096 & 32 & 32 & 3200 \\ \hline
20B & Baseline & 400 & 16 & 98 & 4096 & 32 & 4 & 100 \\ \hline
40B & ZeRO & 400 & 4 & 88 & 6144 & 32 & 12 & 1200 \\ \hline
40B & Baseline & 384 & 32 & 88 & 6144 & 64 & 4 & 48 \\ \hline
60B & ZeRO & 400 & 16 & 132 & 6144 & 32 & 64 & 1600 \\ \hline
60B & Baseline & 384 & 64 & 132 & 6144 & 64 & 4 & 24 \\ \hline
80B & ZeRO & 400 & 16 & 100 & 8192 & 64 & 32 & 800 \\ \hline
80B & Baseline & 384 & 128 & 100 & 8192 & 128 & 4 & 12 \\ \hline
100B & ZeRO & 400 & 16 & 125 & 8192 & 64 & 32 & 800 \\ \hline
100B & Baseline & 384 & 128 & 125 & 8192 & 128 & 2 & 6 \\ \hline
120B & ZeRO & 400 & 16 & 150 & 8192 & 64 & 24 & 600 \\ \hline
120B & Baseline & 384 & 128 & 150 & 8192 & 128 & 2 & 6 \\ \hline
140B & ZeRO & 400 & 16 & 175 & 8192 & 64 & 16 & 400 \\ \hline
140B & Baseline & 384 & 128 & 175 & 8192 & 128 & 2 & 6 \\ \hline
170B & ZeRO & 400 & 16 & 212 & 8192 & 64 & 12 & 300 \\ \hline
170B & Baseline & 256 & 256 & 212 & 8192 & 256 & 2 & 2 \\ \hline
\end{tabular}
\caption{Model parameters and batch sizes to reproduce results in Figure 2 related to ZeRO throughput compared with baseline.} \label{tab:fig2-tab}
\end{table*}

\begin{table*}[!ht]
\begin{tabular}{|l|l|l|l|l|l|l|l|l|}
\hline
\multicolumn{9}{|c|}{Figure 3} \\ \hline
Model size & ZeRO/Baseline & Number of GPUs & MP & Layers & Hidden size & Attention head & Batch size & Total batch size \\ \hline
60B & ZeRO & 64,128,256,400 & 16 & 75 & 8192 & 32 & 16,48,48,64 & 64,384,768,1600 \\ \hline
\end{tabular}
\caption{Model parameters and batch sizes to reproduce results in Figure 3 related to superlinear scalability.} \label{tab:fig3-tab}
\end{table*}

\begin{table*}[!ht]
\begin{tabular}{|l|l|l|l|l|l|l|l|l|}
\hline
\multicolumn{9}{|c|}{Figure 4} \\ \hline
Model size & ZeRO/Baseline & Number of GPUs & MP & Layers & Hidden size & Attention head & Batch size & Total batch size \\ \hline
40B & ZeRO & 400 & 16 & 50 & 8192 & 32 & 16 & 400 \\ \hline
60B & ZeRO & 400 & 16 & 132 & 6144 & 64 & 16 & 400 \\ \hline
140B & ZeRO & 400 & 16 & 175 & 8192 & 64 & 16 & 400 \\ \hline
150B & ZeRO & 400 & 16 & 187 & 8192 & 64 & 16 & 400 \\ \hline
50B & ZeRO & 400 & 16 & 62 & 8192 & 32 & 16 & 400 \\ \hline
\end{tabular}
\caption{Model parameters and batch sizes to reproduce results in Figure 4 related to max model size with different ZeRO configurations.} \label{tab:fig4-tab}
\end{table*}

\begin{table*}[!ht]
\begin{tabular}{|l|l|l|l|l|l|l|l|l|}
\hline
\multicolumn{9}{|c|}{Figure 5} \\ \hline
Model size & ZeRO/Baseline & Number of GPUs & MP & Layers & Hidden size & Attention head & Batch size & Total batch size \\ \hline
40B & ZeRO & 400 & 16 & 50 & 8192 & 32 & 16 & 400 \\ \hline
100B & ZeRO & 400 & 16 & 125 & 8192 & 64 & 32 & 800 \\ \hline
\end{tabular}
\caption{Model parameters and batch sizes to reproduce results in Figure 5 related to memory allocated with different ZeRO configurations.} \label{tab:fig5-tab}
\end{table*}

\begin{table*}[!ht]
\begin{tabular}{|l|l|l|l|l|l|l|l|l|}
\hline
\multicolumn{9}{|c|}{Figure 6} \\ \hline
Model size & ZeRO/Baseline & Number of GPUs & MP & Layers & Hidden size & Attention head & Batch size & Total batch size \\ \hline
60B & ZeRO & 128 & 16 & 75 & 8192 & 64 & 2,4,32,32,8 & 16,32,256,256,64 \\ \hline
170B & ZeRO & 400 & 16 & 212 & 8192 & 64 & 12 & 300 \\ \hline
\end{tabular}
\caption{Model parameters and batch sizes to reproduce results in Figure 6 related to throughput with different ZeRO configurations.} \label{tab:fig6-tab}
\end{table*}

\begin{table*}[!ht]
\begin{tabular}{|l|l|l|l|l|l|l|l|l|}
\hline
\multicolumn{9}{|c|}{Figure 7} \\ \hline
Model size & ZeRO/Baseline & Number of GPUs & MP & Layers & Hidden size & Attention head & Batch size & Total batch size \\ \hline
1.5B & ZeRO & 128 & 1 & 34 & 1920 & 16 & 24 & 3072 \\ \hline
2.5B & ZeRO & 128 & 1 & 54 & 1920 & 16 & 24 & 3072 \\ \hline
4B & ZeRO & 128 & 1 & 64 & 2304 & 24 & 16 & 2048 \\ \hline
6B & ZeRO & 128 & 1 & 52 & 3072 & 24 & 12 & 1536 \\ \hline
8B & ZeRO & 128 & 1 & 72 & 3072 & 24 & 8 & 1024 \\ \hline
10B & ZeRO & 128 & 1 & 50 & 4096 & 32 & 6 & 768 \\ \hline
11B & ZeRO & 128 & 1 & 54 & 4096 & 32 & 4 & 512 \\ \hline
12B & ZeRO & 128 & 1 & 58 & 4096 & 32 & 4 & 512 \\ \hline
13B & ZeRO & 128 & 1 & 62 & 4096 & 32 & 2 & 256 \\ \hline
1p16B & Baseline & 128 & 1 & 24 & 1920 & 16 & 8 & 1024 \\ \hline
1p38B & Baseline & 128 & 1 & 40 & 1536 & 16 & 1 & 128 \\ \hline
\end{tabular}
\caption{Model parameters and batch sizes to reproduce results in Figure 7 related to evaluating maximum model sizes vs throughput while using only data-parallelism.} \label{tab:fig7-tab}
\end{table*}
%STOP_LATEX
